# Supplementary material for: Pollux: Co-adaptive Cluster Scheduling for Goodput-Optimized Deep Learning
Source: arXiv:2008.12260 source file (2021-05-26)
Supplement: Supplementary file 1 [file appendix.tex]

\section{Source Code for the Allocation Search}
\label{sec:allocation-code}

\begin{minted}[fontsize=\tiny]{python}
import numpy as np
import pymoo.model.crossover
import pymoo.model.mutation
import pymoo.model.problem
import pymoo.model.repair
import pymoo.optimize

from pymoo.algorithms.nsga2 import NSGA2
from pymoo.operators.crossover.util import crossover_mask


class Problem(pymoo.model.problem.Problem):
    def __init__(self, jobs, nodes, base_state):
        """
        Multi-objective optimization problem used by PolluxPolicy to determine
        resource allocations and desired cluster size. Optimizes for the best
        performing cluster allocation using only the first N nodes. The cluster
        performance and N are the two objectives being optimized, resulting in
        a set of Pareto-optimal solutions.

        The optimization states are a 3-D array of replica assignments with
        shape (pop_size x num_jobs x num_nodes). The element at k, j, n encodes
        the number of job j replicas assigned to node n, in the kth solution.

        Arguments:
            jobs (list): list of JobInfo objects describing the incomplete jobs
                which need to be scheduled.
            nodes (list): list of NodeInfo objects describing the nodes in the
                cluster, in decreasing order of allocation preference.
            base_state (numpy.array): base optimization state corresponding to
                the current cluster allocations. Shape: (num_jobs x num_nodes).
        """
        assert base_state.shape == (len(jobs), len(nodes))
        self._jobs = jobs
        self._nodes = nodes
        self._base_state = base_state
        # Find which resource types are requested by at least one job.
        rtypes = sorted(set.union(*[set(job.resources) for job in jobs]))
        # Build array of job resources: <num_jobs> x <num_rtypes>. Each entry
        # [j, r] is the amount of resource r requested by a replica of job j.
        self._job_resources = np.zeros((len(jobs), len(rtypes)), np.int64)
        for j, job in enumerate(jobs):
            for r, rtype in enumerate(rtypes):
                self._job_resources[j, r] = job.resources.get(rtype, 0)
        # Build array of node resources: <num_nodes> x <num_rtypes>. Each
        # entry [n, r] is the amount of resource r available on node n.
        self._node_resources = np.zeros((len(nodes), len(rtypes)), np.int64)
        for n, node in enumerate(nodes):
            for r, rtype in enumerate(rtypes):
                self._node_resources[n, r] = node.resources.get(rtype, 0)
        # Calculate dominant per-replica resource shares for each job.
        shares = self._job_resources / np.sum(self._node_resources, axis=0)
        self._dominant_share = np.amax(shares, axis=1)
        # Change base goodput to fair-share goodput.
        fair_replicas = np.ceil(1.0 / self._dominant_share / len(self._jobs))
        fair_nodes = np.ceil(len(nodes) * self._dominant_share)
        for job, num_nodes, num_replicas in zip(jobs, fair_nodes, fair_replicas):
            job.speedup_fn._base_goodput = job.speedup_fn._goodput_fn.optimize(
                num_nodes=num_nodes, num_replicas=num_replicas,
                max_batch_size=job.speedup_fn._max_batch_size,
                atomic_bsz_range=job.speedup_fn._atomic_bsz_range,
                accumulation=job.speedup_fn._accumulation)[0]
        # Upper bound each job: <replicas on node 0> <replicas on node 1> ...
        self._max_replicas = np.zeros(base_state.shape, dtype=np.int)
        for j, job in enumerate(jobs):
            for n, node in enumerate(nodes):
                self._max_replicas[j, n] = min(
                    node.resources[rtype] // job.resources[rtype]
                    for rtype in rtypes if job.resources.get(rtype, 0) > 0)
        super().__init__(n_var=self._base_state.size, n_obj=2, type_var=np.int)

    def get_cluster_utilities(self, states):
        """
        Calculates the cluster utility for each state, defined as the average
        percentage of ideal speedup for each job (ie. speedup / num_replicas),
        weighted by the job's share of the most congested cluster resource.

        Arguments:
            states (numpy.array): a (pop_size x num_jobs x num_nodes) array
                containing the assignments of job replicas to nodes.

        Returns:
            numpy.array: a (pop_size) array containing the utility for each
                state.
        """
        num_replicas = np.sum(states, axis=2)
        speedups = self._get_job_speedups(states)
        # mask (pop_size x num_nodes): indicates which nodes are active.
        mask = np.sum(states, axis=1) > 0
        # total (pop_size x num_rtypes): total amount of cluster resources.
        total = np.sum(np.expand_dims(mask, 2) * self._node_resources, axis=1)
        # alloc (pop_size x num_jobs x num_rtypes):
        #     amount of cluster resources allocated to each job.
        alloc = np.expand_dims(num_replicas, 2) * self._job_resources
        with np.errstate(divide="ignore", invalid="ignore"):
            # shares (pop_size x num_jobs x num_rtypes):
            #     resource shares for each job as a fraction of the cluster.
            shares = np.where(alloc, alloc / np.expand_dims(total, 1), 0.0)
            # utilities (pop_size x num_jobs):
            #     utilities for each job as a fraction of ideal scalability.
            utilities = np.where(num_replicas, speedups / num_replicas, 0.0)
        # Weighted average across all jobs for each rtype.
        utilities = np.sum(np.expand_dims(utilities, 2) * shares, axis=1)
        # Return the utilities for the best utilized rtypes.
        return np.amax(utilities, axis=1)  # Shape: (pop_size).

    def _get_job_speedups(self, states):
        speedup = []
        num_nodes = np.count_nonzero(states, axis=2)
        num_replicas = np.sum(states, axis=2)
        for idx, job in enumerate(self._jobs):
            speedup.append(job.speedup_fn(
                num_nodes[:, idx], num_replicas[:, idx]))
        return np.stack(speedup, axis=1).astype(np.float)

    def _get_cluster_sizes(self, states):
        return np.full(len(states), len(self._nodes))
        #sizes = np.arange(len(self._nodes)) + 1
        #return np.amax(np.where(np.any(states, axis=-2), sizes, 0), axis=-1)

    def _evaluate(self, states, out, *args, **kwargs):
        states = states.reshape(states.shape[0], *self._base_state.shape)
        speedups = self._get_job_speedups(states)
        # Scale the speedup of each job so that a dominant resource share
        # equivalent to a single node results in a speedup of 1.
        scaled_speedups = speedups * self._dominant_share * len(self._nodes)
        # Penalize job restarts.
        num_restarts = np.array([job.num_restarts for job in self._jobs])
        age = np.array([job.age for job in self._jobs])
        delay = 30
        factor = np.maximum(age - num_restarts * delay, 0.0) / (age + delay)
        restart = np.any(states != self._base_state, axis=2)
        scaled_speedups *= np.where(restart, factor, 1)
        p = -1  # Exponent used in power mean. More negative = more fair.
        if p == 0:
            # Geometric mean
            mean = np.exp(np.sum(np.log(np.maximum(scaled_speedups, 1e-3)),
                                 axis=1) / states.shape[1])
        else:
            mean = (np.sum((scaled_speedups + 1e-3) ** p, axis=1)
                    / states.shape[1]) ** (1.0 / p)
        out["F"] = np.column_stack([-mean,
                                    -self.get_cluster_utilities(states)])

    def _crossover(self, states, **kwargs):
        states = states.reshape(*states.shape[:2], *self._base_state.shape)
        n_parents, n_matings, n_jobs, n_nodes = states.shape
        # Single-point crossover over jobs for all parent states.
        points = np.random.randint(n_jobs, size=(n_matings, 1))
        result = crossover_mask(states, np.arange(n_jobs) < points)
        # Set cluster sizes uniformly at random between each pair of parents.
        min_nodes, max_nodes = np.sort(self._get_cluster_sizes(states), axis=0)
        num_nodes = np.random.randint(np.iinfo(np.int16).max,
                                      size=(n_parents, n_matings))
        num_nodes = min_nodes + num_nodes % (max_nodes - min_nodes + 1)
        mask = np.arange(n_nodes) >= np.expand_dims(num_nodes, (2, 3))
        result[np.broadcast_to(mask, result.shape)] = 0
        return result.reshape(n_parents, n_matings, -1)

    def _mutation(self, states, **kwargs):
        states = states.reshape(states.shape[0], *self._base_state.shape)
        # (1) Randomly reset back to base state.
        mask = np.random.random(states.shape[:2]) < 0.1
        states = np.where(np.expand_dims(mask, 2), self._base_state, states)
        # (2) Randomly zero out some elements.
        prob = np.where(np.random.random(states.shape[:2]) < 0.1, 0.1, 0.0)
        states[np.random.random(states.shape) < np.expand_dims(prob, 2)] = 0
        # (3) Randomly increase some elements.
        used_resources = (np.expand_dims(self._job_resources, 1) *
                          np.expand_dims(states, -1)).sum(axis=1)
        free_resources = self._node_resources - used_resources
        mask1 = np.all(np.expand_dims(self._job_resources, 1) <=
                       np.expand_dims(free_resources, 1), axis=-1)
        prob1 = 1.0 * mask1 / np.maximum(mask1.sum(axis=1, keepdims=True), 1.0)
        mask2 = np.logical_and(states, mask1)
        prob2 = 1.0 * mask2 / np.maximum(mask2.sum(axis=1, keepdims=True), 1.0)
        m = np.random.random(states.shape) < prob1 + prob2 - prob1 * prob2
        r = np.random.randint(states, self._max_replicas + 1)
        states[m] = r[m]
        return states.reshape(states.shape[0], -1)

    def _repair(self, pop, **kwargs):
        states = pop.get("X")
        states = states.reshape(states.shape[0], *self._base_state.shape)
        # Copy previous allocations for pinned jobs
        states[:, self._pinned_indices] = \
            self._base_state[self._pinned_indices, :]
        # Order jobs by dominant resource share.
        #sort = np.argsort(self._dominant_share * states.sum(axis=2), axis=1)
        #states = np.take_along_axis(states, np.expand_dims(sort, -1), axis=1)
        # Enforce at most one distributed job per node. Exclude all
        # nonpreemptible jobs.
        distributed = np.count_nonzero(states, axis=2) > 1
        mask = states * np.expand_dims(distributed, axis=-1) > 0
        mask = mask.cumsum(axis=1) > 1
        states[mask] = 0
        # Enforce no more than max replicas per job.
        # max_replicas: (num_jobs x 1)
        max_replicas = np.array([[j.max_replicas] for j in self._jobs])
        shuffle = np.argsort(np.random.random(states.shape), axis=2)
        states = np.take_along_axis(states, shuffle, axis=2)  # Shuffle nodes.
        states = np.minimum(np.cumsum(states, axis=2), max_replicas)
        states = np.diff(states, axis=2, prepend=0)
        max_nodes = 16
        mask = np.minimum(np.cumsum(states > 0, axis=2), max_nodes)
        mask = np.diff(mask, axis=2, prepend=0)
        states[np.logical_not(mask)] = 0
        inverse = np.argsort(shuffle, axis=2)  # Undo shuffle nodes.
        states = np.take_along_axis(states, inverse, axis=2)
        # Enforce node resource limits.
        # job_resources: (num_jobs x num_nodes x num_rtypes)
        job_resources = np.expand_dims(self._job_resources, 1)
        states = np.expand_dims(states, -1) * job_resources
        states = np.minimum(np.cumsum(states, axis=1), self._node_resources)
        states = np.diff(states, axis=1, prepend=0)
        with np.errstate(divide="ignore", invalid="ignore"):
            states = np.amin(np.floor_divide(states, job_resources),
                             where=job_resources > 0, initial=99, axis=-1)
        # Unsort jobs
        #unsort = sort.argsort(axis=1)
        #states = np.take_along_axis(states, np.expand_dims(unsort, -1), axis=1)
        # Only choose solutions which have at least min_replicas allocations
        min_replicas = np.array([j.min_replicas for j in self._jobs])
        mask = np.sum(states, axis=-1) < min_replicas
        states[mask] = 0
        return pop.new("X", states.reshape(states.shape[0], -1))


class Crossover(pymoo.model.crossover.Crossover):
    def __init__(self):
        super().__init__(n_parents=2, n_offsprings=2)

    def _do(self, problem, states, **kwargs):
        return problem._crossover(states, **kwargs)


class Mutation(pymoo.model.mutation.Mutation):
    def _do(self, problem, states, **kwargs):
        return problem._mutation(states, **kwargs)


class Repair(pymoo.model.repair.Repair):
    def _do(self, problem, pop, **kwargs):
        return problem._repair(pop, **kwargs)
\end{minted}
